# Supplementary material for: CEBaB: Estimating the Causal Effects of Real-World Concepts on NLP Model Behavior
Source: arXiv:2205.14140 source file (2022-10-12)
Supplement: Supplementary file 1 [file appendix-results.tex]

\subsection{Binary models with the ICaCE-cosine metric}

\subsubsection{bert-base-uncased (binary, ICaCE-cosine)}
\begin{center}
\begin{tabular}{lllll}
\toprule
{} &       ambiance &           food &          noise &        service \\
\midrule
RandomExplainer &  0.99 (± 0.01) &  0.98 (± 0.04) &  0.99 (± 0.02) &   1.0 (± 0.02) \\
CONEXP          &  0.68 (± 0.05) &  0.45 (± 0.04) &  0.82 (± 0.07) &   0.7 (± 0.04) \\
SLearner        &   0.7 (± 0.05) &  0.49 (± 0.03) &  0.82 (± 0.07) &   0.7 (± 0.03) \\
CausaLM         &  0.86 (± 0.01) &  0.59 (± 0.01) &   0.96 (± 0.0) &  0.82 (± 0.01) \\
TCAV            &   1.01 (± 0.0) &  0.98 (± 0.03) &    1.0 (± 0.0) &   1.0 (± 0.01) \\
INLP            &  0.88 (± 0.01) &  0.59 (± 0.01) &   0.95 (± 0.0) &   0.83 (± 0.0) \\
ConceptShap     &  1.12 (± 0.03) &  1.39 (± 0.05) &  1.04 (± 0.01) &  1.16 (± 0.01) \\
\bottomrule
\end{tabular}
\end{center}

\subsubsection{GPT-2 (binary, ICaCE-cosine)}
\begin{center}
\begin{tabular}{lllll}
\toprule
{} &       ambiance &           food &          noise &        service \\
\midrule
RandomExplainer &  1.01 (± 0.02) &  1.02 (± 0.03) &   1.0 (± 0.02) &  1.01 (± 0.03) \\
CONEXP          &  0.63 (± 0.03) &  0.38 (± 0.02) &  0.81 (± 0.02) &  0.61 (± 0.01) \\
SLearner        &  0.65 (± 0.03) &  0.41 (± 0.01) &  0.82 (± 0.03) &  0.62 (± 0.01) \\
TCAV            &    1.0 (± 0.0) &    1.0 (± 0.0) &    1.0 (± 0.0) &    1.0 (± 0.0) \\
INLP            &    1.0 (± 0.0) &  1.01 (± 0.01) &    1.0 (± 0.0) &    1.0 (± 0.0) \\
ConceptShap     &   1.0 (± 0.01) &  1.05 (± 0.01) &  1.01 (± 0.01) &  1.01 (± 0.01) \\
CausaLM         &  0.82 (± 0.02) &  0.69 (± 0.01) &  0.94 (± 0.02) &  0.79 (± 0.02) \\
\bottomrule
\end{tabular}
\end{center}

\subsubsection{LSTM (binary, ICaCE-cosine)}
\begin{center}
\begin{tabular}{lllll}
\toprule
{} &       ambiance &           food &          noise &        service \\
\midrule
RandomExplainer &  0.98 (± 0.02) &   1.0 (± 0.03) &  1.01 (± 0.03) &   1.0 (± 0.01) \\
CONEXP          &  0.77 (± 0.02) &   0.5 (± 0.01) &  0.88 (± 0.01) &  0.73 (± 0.01) \\
SLearner        &  0.79 (± 0.02) &  0.52 (± 0.01) &  0.88 (± 0.01) &  0.74 (± 0.02) \\
TCAV            &    1.0 (± 0.0) &    1.0 (± 0.0) &    1.0 (± 0.0) &    1.0 (± 0.0) \\
INLP            &  0.89 (± 0.01) &   0.64 (± 0.0) &  0.94 (± 0.01) &  0.83 (± 0.01) \\
ConceptShap     &    1.0 (± 0.0) &    1.0 (± 0.0) &  0.99 (± 0.02) &    1.0 (± 0.0) \\
CausaLM         &    1.0 (± 0.0) &    1.0 (± 0.0) &    1.0 (± 0.0) &    1.0 (± 0.0) \\
\bottomrule
\end{tabular}
\end{center}

\subsubsection{roberta-base (binary, ICaCE-cosine)}
\begin{center}
\begin{tabular}{lllll}
\toprule
{} &       ambiance &           food &          noise &        service \\
\midrule
RandomExplainer &  1.01 (± 0.01) &  1.01 (± 0.03) &  0.99 (± 0.02) &   1.0 (± 0.02) \\
CONEXP          &  0.78 (± 0.02) &  0.47 (± 0.03) &  0.87 (± 0.04) &  0.76 (± 0.03) \\
SLearner        &  0.79 (± 0.02) &   0.5 (± 0.03) &  0.87 (± 0.03) &  0.76 (± 0.03) \\
TCAV            &    1.0 (± 0.0) &    1.0 (± 0.0) &    1.0 (± 0.0) &    1.0 (± 0.0) \\
INLP            &   0.88 (± 0.0) &   0.6 (± 0.01) &  0.95 (± 0.01) &  0.84 (± 0.01) \\
ConceptShap     &  1.09 (± 0.05) &  1.24 (± 0.06) &  1.04 (± 0.02) &  1.09 (± 0.02) \\
CausaLM         &  0.88 (± 0.01) &  0.66 (± 0.01) &  0.95 (± 0.01) &  0.86 (± 0.01) \\
\bottomrule
\end{tabular}
\end{center}

\subsection{Binary models with the ICaCE-L2 metric}

\subsubsection{bert-base-uncased (binary, ICaCE-L2)}
\begin{center}
\begin{tabular}{lllll}
\toprule
{} &       ambiance &           food &          noise &        service \\
\midrule
RandomExplainer &  0.51 (± 0.01) &   0.8 (± 0.01) &  0.44 (± 0.01) &  0.56 (± 0.02) \\
CONEXP          &  0.45 (± 0.01) &   0.58 (± 0.0) &   0.37 (± 0.0) &   0.58 (± 0.0) \\
SLearner        &  0.22 (± 0.01) &  0.44 (± 0.01) &   0.16 (± 0.0) &   0.34 (± 0.0) \\
CausaLM         &   0.3 (± 0.03) &  0.58 (± 0.01) &  0.26 (± 0.02) &  0.36 (± 0.01) \\
TCAV            &  0.19 (± 0.02) &  0.59 (± 0.01) &  0.09 (± 0.01) &  0.25 (± 0.01) \\
INLP            &  0.32 (± 0.06) &   0.7 (± 0.01) &  0.41 (± 0.14) &   0.51 (± 0.1) \\
ConceptShap     &   0.6 (± 0.13) &  1.12 (± 0.12) &  0.42 (± 0.18) &  0.73 (± 0.15) \\
\bottomrule
\end{tabular}
\end{center}

\subsubsection{GPT-2 (binary, ICaCE-L2)}
\begin{center}
\begin{tabular}{lllll}
\toprule
{} &       ambiance &           food &          noise &        service \\
\midrule
RandomExplainer &  0.51 (± 0.01) &    0.8 (± 0.0) &  0.42 (± 0.01) &  0.57 (± 0.01) \\
CONEXP          &  0.44 (± 0.01) &   0.59 (± 0.0) &   0.37 (± 0.0) &   0.57 (± 0.0) \\
SLearner        &  0.22 (± 0.01) &  0.45 (± 0.01) &   0.16 (± 0.0) &  0.35 (± 0.01) \\
TCAV            &   1.48 (± 0.0) &   1.64 (± 0.0) &   1.44 (± 0.0) &   1.51 (± 0.0) \\
INLP            &  0.35 (± 0.12) &  0.64 (± 0.02) &  0.34 (± 0.14) &  0.38 (± 0.05) \\
ConceptShap     &  0.29 (± 0.04) &  0.68 (± 0.04) &  0.13 (± 0.02) &  0.32 (± 0.02) \\
CausaLM         &   0.5 (± 0.02) &  0.68 (± 0.01) &  0.43 (± 0.02) &  0.53 (± 0.01) \\
\bottomrule
\end{tabular}
\end{center}

\subsubsection{LSTM (binary, ICaCE-L2)}
\begin{center}
\begin{tabular}{lllll}
\toprule
{} &       ambiance &           food &          noise &        service \\
\midrule
RandomExplainer &   0.5 (± 0.01) &  0.75 (± 0.02) &  0.44 (± 0.02) &  0.57 (± 0.01) \\
CONEXP          &  0.45 (± 0.01) &    0.6 (± 0.0) &   0.37 (± 0.0) &   0.57 (± 0.0) \\
SLearner        &  0.23 (± 0.01) &  0.46 (± 0.01) &  0.16 (± 0.01) &  0.35 (± 0.01) \\
TCAV            &  1.48 (± 0.01) &   1.62 (± 0.0) &   1.44 (± 0.0) &   1.52 (± 0.0) \\
INLP            &  0.21 (± 0.04) &   0.7 (± 0.01) &  0.08 (± 0.01) &   0.7 (± 0.04) \\
ConceptShap     &  0.79 (± 0.01) &  0.92 (± 0.06) &  0.64 (± 0.19) &  0.72 (± 0.11) \\
CausaLM         &  0.18 (± 0.02) &  0.52 (± 0.01) &  0.08 (± 0.01) &  0.26 (± 0.01) \\
\bottomrule
\end{tabular}
\end{center}

\subsubsection{roberta-base (binary, ICaCE-L2)}
\begin{center}
\begin{tabular}{lllll}
\toprule
{} &       ambiance &           food &          noise &        service \\
\midrule
RandomExplainer &  0.51 (± 0.01) &   0.8 (± 0.01) &  0.44 (± 0.02) &  0.55 (± 0.01) \\
CONEXP          &   0.45 (± 0.0) &   0.59 (± 0.0) &  0.37 (± 0.01) &   0.58 (± 0.0) \\
SLearner        &  0.22 (± 0.01) &  0.45 (± 0.01) &  0.16 (± 0.01) &  0.34 (± 0.01) \\
TCAV            &   1.49 (± 0.0) &   1.65 (± 0.0) &   1.44 (± 0.0) &   1.51 (± 0.0) \\
INLP            &  0.17 (± 0.01) &  0.65 (± 0.01) &  0.08 (± 0.02) &  0.23 (± 0.01) \\
ConceptShap     &  0.59 (± 0.23) &  0.92 (± 0.15) &  0.55 (± 0.11) &  0.58 (± 0.09) \\
CausaLM         &   0.58 (± 0.0) &  0.71 (± 0.01) &  0.55 (± 0.01) &  0.57 (± 0.01) \\
\bottomrule
\end{tabular}
\end{center}

\subsection{Binary models with the ICaCE-normdiff metric}

\subsubsection{bert-base-uncased (binary, ICaCE-normdiff)}
\begin{center}
\begin{tabular}{lllll}
\toprule
{} &       ambiance &           food &          noise &        service \\
\midrule
RandomExplainer &  0.46 (± 0.01) &  0.65 (± 0.01) &  0.42 (± 0.01) &  0.49 (± 0.02) \\
CONEXP          &  0.45 (± 0.01) &   0.57 (± 0.0) &   0.37 (± 0.0) &   0.57 (± 0.0) \\
SLearner        &  0.22 (± 0.01) &  0.43 (± 0.01) &   0.16 (± 0.0) &   0.34 (± 0.0) \\
CausaLM         &   0.3 (± 0.03) &  0.57 (± 0.01) &  0.25 (± 0.02) &  0.35 (± 0.02) \\
TCAV            &  0.19 (± 0.02) &  0.58 (± 0.01) &  0.09 (± 0.01) &  0.25 (± 0.01) \\
INLP            &  0.32 (± 0.06) &  0.69 (± 0.01) &  0.41 (± 0.14) &   0.51 (± 0.1) \\
ConceptShap     &   0.51 (± 0.1) &  0.68 (± 0.01) &  0.39 (± 0.17) &   0.56 (± 0.1) \\
\bottomrule
\end{tabular}
\end{center}

\subsubsection{GPT-2 (binary, ICaCE-normdiff)}
\begin{center}
\begin{tabular}{lllll}
\toprule
{} &       ambiance &           food &          noise &        service \\
\midrule
RandomExplainer &  0.45 (± 0.01) &  0.63 (± 0.01) &  0.41 (± 0.01) &   0.5 (± 0.01) \\
CONEXP          &  0.44 (± 0.01) &   0.58 (± 0.0) &   0.36 (± 0.0) &   0.56 (± 0.0) \\
SLearner        &  0.22 (± 0.01) &   0.45 (± 0.0) &   0.15 (± 0.0) &  0.34 (± 0.01) \\
TCAV            &  1.25 (± 0.01) &  0.87 (± 0.01) &   1.35 (± 0.0) &   1.17 (± 0.0) \\
INLP            &   0.32 (± 0.1) &  0.58 (± 0.01) &  0.33 (± 0.13) &  0.35 (± 0.04) \\
ConceptShap     &  0.27 (± 0.04) &   0.6 (± 0.02) &  0.13 (± 0.02) &   0.3 (± 0.01) \\
CausaLM         &  0.49 (± 0.02) &  0.64 (± 0.01) &  0.43 (± 0.02) &  0.52 (± 0.01) \\
\bottomrule
\end{tabular}
\end{center}

\subsubsection{LSTM (binary, ICaCE-normdiff)}
\begin{center}
\begin{tabular}{lllll}
\toprule
{} &       ambiance &           food &          noise &        service \\
\midrule
RandomExplainer &  0.45 (± 0.01) &   0.6 (± 0.01) &  0.41 (± 0.02) &  0.49 (± 0.01) \\
CONEXP          &  0.44 (± 0.01) &    0.6 (± 0.0) &   0.36 (± 0.0) &  0.56 (± 0.01) \\
SLearner        &  0.23 (± 0.01) &  0.45 (± 0.01) &  0.16 (± 0.01) &  0.35 (± 0.01) \\
TCAV            &  1.24 (± 0.02) &   0.9 (± 0.01) &  1.34 (± 0.01) &  1.16 (± 0.01) \\
INLP            &   0.2 (± 0.04) &  0.69 (± 0.01) &  0.07 (± 0.01) &  0.69 (± 0.04) \\
ConceptShap     &   0.69 (± 0.0) &  0.67 (± 0.03) &   0.6 (± 0.17) &  0.61 (± 0.08) \\
CausaLM         &  0.18 (± 0.02) &  0.52 (± 0.01) &  0.08 (± 0.01) &  0.26 (± 0.01) \\
\bottomrule
\end{tabular}
\end{center}

\subsubsection{roberta-base (binary, ICaCE-normdiff)}
\begin{center}
\begin{tabular}{lllll}
\toprule
{} &       ambiance &           food &          noise &        service \\
\midrule
RandomExplainer &  0.47 (± 0.01) &  0.65 (± 0.01) &  0.42 (± 0.01) &  0.49 (± 0.01) \\
CONEXP          &   0.45 (± 0.0) &   0.59 (± 0.0) &  0.37 (± 0.01) &   0.57 (± 0.0) \\
SLearner        &  0.22 (± 0.01) &  0.44 (± 0.01) &  0.16 (± 0.01) &  0.34 (± 0.01) \\
TCAV            &  1.24 (± 0.01) &  0.85 (± 0.01) &  1.34 (± 0.01) &  1.19 (± 0.01) \\
INLP            &  0.17 (± 0.01) &  0.65 (± 0.01) &  0.08 (± 0.02) &  0.23 (± 0.01) \\
ConceptShap     &   0.5 (± 0.17) &  0.64 (± 0.04) &   0.51 (± 0.1) &  0.48 (± 0.06) \\
CausaLM         &   0.58 (± 0.0) &   0.69 (± 0.0) &  0.55 (± 0.01) &  0.56 (± 0.01) \\
\bottomrule
\end{tabular}
\end{center}

\subsection{3-way models with the ICaCE-cosine metric}

\subsubsection{bert-base-uncased (3-way, ICaCE-cosine)}
\begin{center}
\begin{tabular}{lllll}
\toprule
{} &       ambiance &           food &          noise &        service \\
\midrule
RandomExplainer &   1.0 (± 0.03) &  0.98 (± 0.01) &  1.01 (± 0.02) &  0.99 (± 0.03) \\
CONEXP          &  0.68 (± 0.06) &  0.52 (± 0.02) &  0.79 (± 0.08) &  0.66 (± 0.04) \\
SLearner        &  0.57 (± 0.04) &  0.46 (± 0.02) &  0.67 (± 0.07) &  0.51 (± 0.04) \\
TCAV            &    1.0 (± 0.0) &    1.0 (± 0.0) &    1.0 (± 0.0) &    1.0 (± 0.0) \\
INLP            &  0.74 (± 0.01) &  0.57 (± 0.02) &  0.86 (± 0.02) &   0.7 (± 0.01) \\
ConceptShap     &  1.16 (± 0.03) &  1.32 (± 0.02) &  1.07 (± 0.03) &  1.19 (± 0.03) \\
CausaLM         &  0.78 (± 0.03) &  0.69 (± 0.01) &  0.88 (± 0.02) &  0.76 (± 0.01) \\
\bottomrule
\end{tabular}
\end{center}

\subsubsection{GPT-2 (3-way, ICaCE-cosine)}
\begin{center}
\begin{tabular}{lllll}
\toprule
{} &       ambiance &           food &          noise &        service \\
\midrule
RandomExplainer &   1.0 (± 0.01) &  1.01 (± 0.02) &   1.0 (± 0.03) &   1.0 (± 0.02) \\
CONEXP          &  0.63 (± 0.02) &  0.49 (± 0.01) &  0.73 (± 0.03) &  0.59 (± 0.01) \\
SLearner        &  0.56 (± 0.02) &  0.45 (± 0.02) &  0.59 (± 0.02) &  0.45 (± 0.01) \\
TCAV            &    1.0 (± 0.0) &    1.0 (± 0.0) &    1.0 (± 0.0) &    1.0 (± 0.0) \\
INLP            &    1.0 (± 0.0) &    1.0 (± 0.0) &    1.0 (± 0.0) &    1.0 (± 0.0) \\
ConceptShap     &   1.01 (± 0.0) &  1.02 (± 0.01) &    1.0 (± 0.0) &    1.0 (± 0.0) \\
CausaLM         &  0.77 (± 0.01) &  0.76 (± 0.01) &  0.85 (± 0.01) &   0.8 (± 0.01) \\
\bottomrule
\end{tabular}
\end{center}

\subsubsection{LSTM (3-way, ICaCE-cosine)}
\begin{center}
\begin{tabular}{lllll}
\toprule
{} &       ambiance &           food &          noise &        service \\
\midrule
RandomExplainer &  1.01 (± 0.02) &  0.99 (± 0.02) &  0.99 (± 0.01) &  1.01 (± 0.01) \\
CONEXP          &   0.64 (± 0.0) &  0.55 (± 0.01) &  0.75 (± 0.01) &  0.65 (± 0.01) \\
SLearner        &  0.61 (± 0.01) &  0.53 (± 0.01) &  0.72 (± 0.02) &  0.59 (± 0.01) \\
TCAV            &    1.0 (± 0.0) &    1.0 (± 0.0) &    1.0 (± 0.0) &    1.0 (± 0.0) \\
INLP            &  0.86 (± 0.07) &  0.67 (± 0.02) &  0.93 (± 0.08) &  0.76 (± 0.02) \\
ConceptShap     &  1.01 (± 0.01) &  1.02 (± 0.04) &    1.0 (± 0.0) &    1.0 (± 0.0) \\
CausaLM         &    1.0 (± 0.0) &    1.0 (± 0.0) &    1.0 (± 0.0) &    1.0 (± 0.0) \\
\bottomrule
\end{tabular}
\end{center}

\subsubsection{roberta-base (3-way, ICaCE-cosine)}
\begin{center}
\begin{tabular}{lllll}
\toprule
{} &       ambiance &           food &          noise &        service \\
\midrule
RandomExplainer &  1.01 (± 0.02) &   1.0 (± 0.02) &    1.0 (± 0.0) &   1.0 (± 0.02) \\
CONEXP          &  0.79 (± 0.03) &  0.57 (± 0.02) &  0.91 (± 0.03) &  0.76 (± 0.05) \\
SLearner        &  0.66 (± 0.02) &  0.51 (± 0.02) &   0.8 (± 0.02) &  0.62 (± 0.04) \\
TCAV            &    1.0 (± 0.0) &    1.0 (± 0.0) &    1.0 (± 0.0) &    1.0 (± 0.0) \\
INLP            &  0.77 (± 0.02) &   0.6 (± 0.02) &  0.84 (± 0.02) &  0.74 (± 0.01) \\
ConceptShap     &  1.09 (± 0.02) &  1.19 (± 0.05) &  1.06 (± 0.02) &   1.1 (± 0.02) \\
CausaLM         &  0.81 (± 0.01) &   0.68 (± 0.0) &  0.89 (± 0.01) &  0.76 (± 0.01) \\
\bottomrule
\end{tabular}
\end{center}

\subsection{3-way models with the ICaCE-L2 metric}

\subsubsection{bert-base-uncased (3-way, ICaCE-L2)}
\begin{center}
\begin{tabular}{lllll}
\toprule
{} &       ambiance &           food &          noise &        service \\
\midrule
RandomExplainer &  0.71 (± 0.01) &  0.95 (± 0.01) &  0.57 (± 0.02) &  0.77 (± 0.01) \\
CONEXP          &  0.58 (± 0.01) &   0.79 (± 0.0) &  0.42 (± 0.02) &   0.66 (± 0.0) \\
SLearner        &  0.51 (± 0.01) &  0.69 (± 0.01) &  0.35 (± 0.02) &  0.58 (± 0.01) \\
TCAV            &   1.88 (± 0.0) &    2.0 (± 0.0) &  1.81 (± 0.01) &   1.91 (± 0.0) \\
INLP            &  0.46 (± 0.01) &   0.8 (± 0.02) &  0.33 (± 0.06) &  0.56 (± 0.02) \\
ConceptShap     &  0.81 (± 0.06) &   1.2 (± 0.04) &   0.6 (± 0.07) &  0.95 (± 0.07) \\
CausaLM         &  0.67 (± 0.01) &  0.84 (± 0.01) &  0.55 (± 0.02) &   0.7 (± 0.01) \\
\bottomrule
\end{tabular}
\end{center}

\subsubsection{GPT-2 (3-way, ICaCE-L2)}
\begin{center}
\begin{tabular}{lllll}
\toprule
{} &       ambiance &           food &          noise &        service \\
\midrule
RandomExplainer &  0.67 (± 0.01) &  0.92 (± 0.01) &  0.54 (± 0.01) &  0.73 (± 0.01) \\
CONEXP          &  0.51 (± 0.01) &  0.75 (± 0.01) &  0.38 (± 0.01) &  0.61 (± 0.01) \\
SLearner        &  0.45 (± 0.01) &  0.65 (± 0.01) &  0.31 (± 0.01) &  0.53 (± 0.01) \\
TCAV            &   1.85 (± 0.0) &  1.97 (± 0.01) &   1.79 (± 0.0) &   1.89 (± 0.0) \\
INLP            &  0.52 (± 0.08) &    0.8 (± 0.0) &  0.34 (± 0.06) &  0.61 (± 0.08) \\
ConceptShap     &  0.61 (± 0.01) &  0.89 (± 0.01) &  0.46 (± 0.01) &   0.67 (± 0.0) \\
CausaLM         &  0.62 (± 0.01) &  0.82 (± 0.01) &  0.52 (± 0.01) &  0.67 (± 0.01) \\
\bottomrule
\end{tabular}
\end{center}

\subsubsection{LSTM (3-way, ICaCE-L2)}
\begin{center}
\begin{tabular}{lllll}
\toprule
{} &       ambiance &           food &          noise &        service \\
\midrule
RandomExplainer &  0.72 (± 0.01) &   0.9 (± 0.01) &  0.57 (± 0.02) &  0.74 (± 0.01) \\
CONEXP          &  0.57 (± 0.01) &  0.76 (± 0.01) &  0.43 (± 0.02) &  0.63 (± 0.01) \\
SLearner        &  0.51 (± 0.01) &  0.67 (± 0.01) &  0.37 (± 0.02) &  0.56 (± 0.01) \\
TCAV            &   1.88 (± 0.0) &   1.97 (± 0.0) &  1.81 (± 0.01) &   1.89 (± 0.0) \\
INLP            &  0.48 (± 0.02) &  0.88 (± 0.01) &  0.28 (± 0.02) &  0.84 (± 0.03) \\
ConceptShap     &  0.99 (± 0.08) &  1.11 (± 0.06) &  0.88 (± 0.06) &  1.06 (± 0.03) \\
CausaLM         &  0.46 (± 0.01) &  0.71 (± 0.01) &  0.28 (± 0.03) &   0.5 (± 0.01) \\
\bottomrule
\end{tabular}
\end{center}

\subsubsection{roberta-base (3-way, ICaCE-L2)}
\begin{center}
\begin{tabular}{lllll}
\toprule
{} &       ambiance &           food &          noise &        service \\
\midrule
RandomExplainer &   0.7 (± 0.02) &  0.98 (± 0.01) &   0.6 (± 0.01) &  0.74 (± 0.01) \\
CONEXP          &  0.56 (± 0.01) &  0.81 (± 0.01) &  0.46 (± 0.01) &  0.64 (± 0.01) \\
SLearner        &   0.5 (± 0.01) &  0.71 (± 0.01) &  0.38 (± 0.01) &  0.57 (± 0.01) \\
TCAV            &  1.88 (± 0.01) &   2.01 (± 0.0) &   1.83 (± 0.0) &   1.9 (± 0.01) \\
INLP            &  0.42 (± 0.02) &   0.8 (± 0.01) &   0.29 (± 0.0) &  0.49 (± 0.02) \\
ConceptShap     &  0.78 (± 0.05) &  1.12 (± 0.07) &  0.67 (± 0.03) &   0.8 (± 0.04) \\
CausaLM         &  0.69 (± 0.01) &  0.87 (± 0.01) &  0.62 (± 0.01) &  0.69 (± 0.01) \\
\bottomrule
\end{tabular}
\end{center}

\subsection{3-way models with the ICaCE-normdiff metric}

\subsubsection{bert-base-uncased (3-way, ICaCE-normdiff)}
\begin{center}
\begin{tabular}{lllll}
\toprule
{} &       ambiance &           food &          noise &        service \\
\midrule
RandomExplainer &  0.56 (± 0.01) &   0.7 (± 0.01) &  0.47 (± 0.01) &   0.59 (± 0.0) \\
CONEXP          &  0.51 (± 0.01) &   0.62 (± 0.0) &  0.39 (± 0.01) &   0.56 (± 0.0) \\
SLearner        &  0.47 (± 0.01) &  0.54 (± 0.01) &  0.32 (± 0.01) &  0.51 (± 0.01) \\
TCAV            &  1.28 (± 0.01) &  0.96 (± 0.01) &  1.48 (± 0.02) &   1.2 (± 0.01) \\
INLP            &  0.45 (± 0.01) &   0.75 (± 0.0) &  0.31 (± 0.06) &  0.54 (± 0.02) \\
ConceptShap     &  0.58 (± 0.03) &    0.7 (± 0.0) &  0.48 (± 0.06) &  0.64 (± 0.02) \\
CausaLM         &   0.59 (± 0.0) &  0.73 (± 0.01) &   0.5 (± 0.01) &  0.61 (± 0.01) \\
\bottomrule
\end{tabular}
\end{center}

\subsubsection{GPT-2 (3-way, ICaCE-normdiff)}
\begin{center}
\begin{tabular}{lllll}
\toprule
{} &       ambiance &           food &          noise &        service \\
\midrule
RandomExplainer &   0.5 (± 0.01) &  0.64 (± 0.01) &  0.41 (± 0.01) &  0.53 (± 0.01) \\
CONEXP          &  0.44 (± 0.01) &  0.55 (± 0.01) &  0.33 (± 0.01) &   0.49 (± 0.0) \\
SLearner        &  0.41 (± 0.01) &  0.48 (± 0.01) &  0.27 (± 0.01) &  0.45 (± 0.01) \\
TCAV            &  1.33 (± 0.01) &  0.99 (± 0.01) &  1.49 (± 0.01) &   1.23 (± 0.0) \\
INLP            &  0.43 (± 0.03) &  0.68 (± 0.02) &  0.28 (± 0.04) &   0.5 (± 0.01) \\
ConceptShap     &  0.46 (± 0.01) &  0.65 (± 0.01) &  0.35 (± 0.01) &  0.51 (± 0.01) \\
CausaLM         &   0.52 (± 0.0) &  0.64 (± 0.01) &  0.43 (± 0.01) &  0.53 (± 0.01) \\
\bottomrule
\end{tabular}
\end{center}

\subsubsection{LSTM (3-way, ICaCE-normdiff)}
\begin{center}
\begin{tabular}{lllll}
\toprule
{} &       ambiance &           food &          noise &        service \\
\midrule
RandomExplainer &  0.54 (± 0.01) &  0.65 (± 0.01) &  0.45 (± 0.01) &  0.55 (± 0.01) \\
CONEXP          &  0.49 (± 0.01) &   0.58 (± 0.0) &  0.38 (± 0.02) &  0.52 (± 0.01) \\
SLearner        &  0.46 (± 0.01) &   0.51 (± 0.0) &  0.33 (± 0.02) &  0.48 (± 0.01) \\
TCAV            &  1.27 (± 0.01) &  1.02 (± 0.01) &  1.45 (± 0.03) &  1.23 (± 0.01) \\
INLP            &  0.41 (± 0.02) &   0.7 (± 0.01) &  0.25 (± 0.02) &  0.72 (± 0.03) \\
ConceptShap     &  0.65 (± 0.04) &  0.63 (± 0.01) &  0.66 (± 0.05) &  0.66 (± 0.01) \\
CausaLM         &  0.46 (± 0.01) &  0.71 (± 0.01) &  0.28 (± 0.03) &   0.5 (± 0.01) \\
\bottomrule
\end{tabular}
\end{center}

\subsubsection{roberta-base (3-way, ICaCE-normdiff)}
\begin{center}
\begin{tabular}{lllll}
\toprule
{} &       ambiance &           food &          noise &        service \\
\midrule
RandomExplainer &  0.55 (± 0.01) &  0.73 (± 0.01) &  0.49 (± 0.01) &  0.58 (± 0.01) \\
CONEXP          &   0.5 (± 0.01) &   0.63 (± 0.0) &  0.42 (± 0.01) &  0.55 (± 0.01) \\
SLearner        &  0.46 (± 0.01) &  0.54 (± 0.01) &   0.34 (± 0.0) &  0.51 (± 0.01) \\
TCAV            &  1.31 (± 0.02) &  0.94 (± 0.01) &   1.44 (± 0.0) &  1.24 (± 0.02) \\
INLP            &  0.42 (± 0.02) &  0.78 (± 0.01) &  0.29 (± 0.01) &  0.48 (± 0.02) \\
ConceptShap     &  0.57 (± 0.03) &  0.71 (± 0.01) &  0.53 (± 0.03) &  0.58 (± 0.01) \\
CausaLM         &  0.62 (± 0.01) &  0.76 (± 0.01) &  0.57 (± 0.01) &  0.62 (± 0.01) \\
\bottomrule
\end{tabular}
\end{center}

\subsection{5-way models with the ICaCE-cosine metric}

\subsubsection{bert-base-uncased (5-way, ICaCE-cosine)}
\begin{center}
\begin{tabular}{lllll}
\toprule
{} &       ambiance &           food &          noise &        service \\
\midrule
RandomExplainer &   1.0 (± 0.01) &   1.0 (± 0.01) &   1.0 (± 0.02) &   1.0 (± 0.01) \\
CONEXP          &  0.72 (± 0.01) &  0.72 (± 0.02) &  0.71 (± 0.01) &  0.74 (± 0.02) \\
SLearner        &  0.63 (± 0.02) &  0.65 (± 0.02) &   0.6 (± 0.02) &  0.62 (± 0.02) \\
TCAV            &    1.0 (± 0.0) &    1.0 (± 0.0) &    1.0 (± 0.0) &    1.0 (± 0.0) \\
INLP            &  0.57 (± 0.04) &  0.57 (± 0.04) &  0.64 (± 0.03) &   0.6 (± 0.01) \\
ConceptShap     &   1.1 (± 0.02) &  1.17 (± 0.02) &  1.06 (± 0.02) &  1.09 (± 0.03) \\
CausaLM         &   0.78 (± 0.0) &  0.76 (± 0.01) &   0.84 (± 0.0) &  0.79 (± 0.01) \\
\bottomrule
\end{tabular}
\end{center}

\subsubsection{GPT-2 (5-way, ICaCE-cosine)}
\begin{center}
\begin{tabular}{lllll}
\toprule
{} &       ambiance &           food &          noise &        service \\
\midrule
RandomExplainer &  1.01 (± 0.01) &   1.0 (± 0.01) &   1.0 (± 0.03) &   1.0 (± 0.02) \\
CONEXP          &  0.68 (± 0.01) &  0.63 (± 0.01) &  0.71 (± 0.01) &  0.69 (± 0.01) \\
SLearner        &  0.65 (± 0.02) &  0.57 (± 0.01) &  0.57 (± 0.03) &  0.58 (± 0.01) \\
TCAV            &    1.0 (± 0.0) &    1.0 (± 0.0) &    1.0 (± 0.0) &    1.0 (± 0.0) \\
INLP            &    1.0 (± 0.0) &   1.0 (± 0.01) &    1.0 (± 0.0) &    1.0 (± 0.0) \\
ConceptShap     &    1.0 (± 0.0) &    1.0 (± 0.0) &    1.0 (± 0.0) &    1.0 (± 0.0) \\
CausaLM         &   0.81 (± 0.0) &   0.8 (± 0.01) &  0.85 (± 0.01) &  0.84 (± 0.01) \\
\bottomrule
\end{tabular}
\end{center}

\subsubsection{LSTM (5-way, ICaCE-cosine)}
\begin{center}
\begin{tabular}{lllll}
\toprule
{} &       ambiance &           food &          noise &        service \\
\midrule
RandomExplainer &   1.0 (± 0.02) &   1.0 (± 0.01) &   1.0 (± 0.01) &   1.0 (± 0.01) \\
CONEXP          &    0.7 (± 0.0) &  0.72 (± 0.01) &  0.71 (± 0.01) &  0.72 (± 0.01) \\
SLearner        &  0.64 (± 0.01) &  0.67 (± 0.01) &  0.59 (± 0.01) &  0.62 (± 0.01) \\
TCAV            &    1.0 (± 0.0) &    1.0 (± 0.0) &    1.0 (± 0.0) &    1.0 (± 0.0) \\
INLP            &  0.78 (± 0.04) &  0.77 (± 0.04) &  0.73 (± 0.03) &  0.67 (± 0.02) \\
ConceptShap     &    1.0 (± 0.0) &    1.0 (± 0.0) &   1.0 (± 0.01) &    1.0 (± 0.0) \\
CausaLM         &    1.0 (± 0.0) &    1.0 (± 0.0) &    1.0 (± 0.0) &    1.0 (± 0.0) \\
\bottomrule
\end{tabular}
\end{center}

\subsubsection{roberta-base (5-way, ICaCE-cosine)}
\begin{center}
\begin{tabular}{lllll}
\toprule
{} &       ambiance &           food &          noise &        service \\
\midrule
RandomExplainer &  0.98 (± 0.02) &   1.0 (± 0.02) &  1.02 (± 0.01) &  0.99 (± 0.01) \\
CONEXP          &   0.72 (± 0.0) &  0.72 (± 0.01) &  0.73 (± 0.01) &  0.78 (± 0.01) \\
SLearner        &  0.64 (± 0.01) &  0.66 (± 0.02) &  0.62 (± 0.01) &  0.65 (± 0.02) \\
TCAV            &    1.0 (± 0.0) &    1.0 (± 0.0) &    1.0 (± 0.0) &    1.0 (± 0.0) \\
INLP            &   0.6 (± 0.02) &  0.52 (± 0.02) &  0.65 (± 0.03) &   0.6 (± 0.01) \\
ConceptShap     &  1.06 (± 0.03) &  1.09 (± 0.02) &  1.03 (± 0.03) &   1.03 (± 0.0) \\
CausaLM         &  0.79 (± 0.01) &  0.72 (± 0.01) &   0.83 (± 0.0) &   0.76 (± 0.0) \\
\bottomrule
\end{tabular}
\end{center}

\subsection{5-way models with the ICaCE-L2 metric}

\subsubsection{bert-base-uncased (5-way, ICaCE-L2)}
\begin{center}
\begin{tabular}{lllll}
\toprule
{} &       ambiance &           food &          noise &        service \\
\midrule
RandomExplainer &  0.93 (± 0.02) &  1.03 (± 0.01) &  0.77 (± 0.02) &  0.93 (± 0.02) \\
CONEXP          &   0.8 (± 0.02) &  0.93 (± 0.01) &  0.65 (± 0.01) &  0.82 (± 0.02) \\
SLearner        &  0.72 (± 0.02) &  0.84 (± 0.01) &  0.58 (± 0.02) &  0.74 (± 0.02) \\
TCAV            &  2.44 (± 0.01) &  2.48 (± 0.01) &  2.38 (± 0.01) &  2.44 (± 0.01) \\
INLP            &  0.79 (± 0.03) &  0.89 (± 0.02) &  0.65 (± 0.01) &   0.8 (± 0.02) \\
ConceptShap     &  1.23 (± 0.03) &  1.39 (± 0.02) &  1.06 (± 0.02) &  1.22 (± 0.02) \\
CausaLM         &  0.87 (± 0.02) &  0.94 (± 0.01) &  0.73 (± 0.02) &  0.85 (± 0.02) \\
\bottomrule
\end{tabular}
\end{center}

\subsubsection{GPT-2 (5-way, ICaCE-L2)}
\begin{center}
\begin{tabular}{lllll}
\toprule
{} &       ambiance &           food &          noise &        service \\
\midrule
RandomExplainer &  0.78 (± 0.02) &   0.9 (± 0.02) &  0.67 (± 0.01) &   0.8 (± 0.02) \\
CONEXP          &  0.65 (± 0.02) &  0.78 (± 0.03) &  0.54 (± 0.02) &  0.68 (± 0.02) \\
SLearner        &  0.57 (± 0.01) &  0.69 (± 0.03) &  0.47 (± 0.02) &   0.6 (± 0.02) \\
TCAV            &  2.38 (± 0.01) &  2.42 (± 0.01) &  2.34 (± 0.01) &  2.38 (± 0.01) \\
INLP            &  0.71 (± 0.03) &  0.82 (± 0.02) &  0.56 (± 0.02) &  0.72 (± 0.01) \\
ConceptShap     &  1.01 (± 0.02) &  1.11 (± 0.02) &  0.92 (± 0.01) &  1.02 (± 0.01) \\
CausaLM         &  0.74 (± 0.02) &  0.83 (± 0.02) &  0.63 (± 0.02) &  0.76 (± 0.01) \\
\bottomrule
\end{tabular}
\end{center}

\subsubsection{LSTM (5-way, ICaCE-L2)}
\begin{center}
\begin{tabular}{lllll}
\toprule
{} &       ambiance &           food &          noise &        service \\
\midrule
RandomExplainer &  0.87 (± 0.02) &  0.97 (± 0.01) &  0.77 (± 0.02) &  0.88 (± 0.01) \\
CONEXP          &  0.75 (± 0.02) &  0.89 (± 0.01) &  0.65 (± 0.02) &  0.78 (± 0.01) \\
SLearner        &   0.7 (± 0.01) &  0.83 (± 0.01) &  0.59 (± 0.02) &  0.73 (± 0.01) \\
TCAV            &  2.42 (± 0.01) &   2.45 (± 0.0) &  2.38 (± 0.01) &   2.42 (± 0.0) \\
INLP            &  0.74 (± 0.03) &   0.9 (± 0.01) &  0.61 (± 0.02) &  0.82 (± 0.02) \\
ConceptShap     &  1.24 (± 0.05) &  1.32 (± 0.04) &  1.21 (± 0.06) &  1.27 (± 0.06) \\
CausaLM         &  0.73 (± 0.02) &  0.86 (± 0.01) &  0.61 (± 0.02) &  0.74 (± 0.01) \\
\bottomrule
\end{tabular}
\end{center}

\subsubsection{roberta-base (5-way, ICaCE-L2)}
\begin{center}
\begin{tabular}{lllll}
\toprule
{} &       ambiance &           food &          noise &        service \\
\midrule
RandomExplainer &  0.94 (± 0.02) &  1.08 (± 0.01) &  0.86 (± 0.02) &  0.95 (± 0.01) \\
CONEXP          &  0.81 (± 0.01) &  0.98 (± 0.01) &  0.75 (± 0.02) &  0.84 (± 0.01) \\
SLearner        &  0.73 (± 0.01) &  0.89 (± 0.01) &  0.67 (± 0.02) &  0.76 (± 0.01) \\
TCAV            &   2.45 (± 0.0) &    2.5 (± 0.0) &  2.42 (± 0.01) &   2.45 (± 0.0) \\
INLP            &  0.79 (± 0.01) &  0.95 (± 0.01) &  0.72 (± 0.02) &  0.81 (± 0.02) \\
ConceptShap     &  1.21 (± 0.03) &  1.35 (± 0.03) &  1.12 (± 0.03) &    1.2 (± 0.0) \\
CausaLM         &  0.88 (± 0.01) &  0.98 (± 0.01) &  0.82 (± 0.02) &  0.88 (± 0.01) \\
\bottomrule
\end{tabular}
\end{center}

\subsection{5-way models with the ICaCE-normdiff metric}

\subsubsection{bert-base-uncased (5-way, ICaCE-normdiff)}
\begin{center}
\begin{tabular}{lllll}
\toprule
{} &       ambiance &           food &          noise &        service \\
\midrule
RandomExplainer &  0.66 (± 0.03) &  0.74 (± 0.01) &  0.53 (± 0.02) &  0.67 (± 0.02) \\
CONEXP          &  0.66 (± 0.02) &  0.65 (± 0.02) &  0.52 (± 0.02) &  0.63 (± 0.02) \\
SLearner        &  0.58 (± 0.02) &  0.55 (± 0.02) &  0.47 (± 0.02) &  0.53 (± 0.02) \\
TCAV            &  1.44 (± 0.02) &  1.32 (± 0.01) &  1.62 (± 0.01) &  1.44 (± 0.02) \\
INLP            &  0.73 (± 0.02) &  0.81 (± 0.02) &  0.56 (± 0.01) &  0.73 (± 0.02) \\
ConceptShap     &  0.58 (± 0.02) &  0.56 (± 0.02) &  0.55 (± 0.03) &  0.57 (± 0.02) \\
CausaLM         &  0.68 (± 0.02) &  0.76 (± 0.02) &  0.55 (± 0.02) &  0.68 (± 0.02) \\
\bottomrule
\end{tabular}
\end{center}

\subsubsection{GPT-2 (5-way, ICaCE-normdiff)}
\begin{center}
\begin{tabular}{lllll}
\toprule
{} &       ambiance &           food &          noise &        service \\
\midrule
RandomExplainer &   0.5 (± 0.03) &  0.59 (± 0.02) &  0.41 (± 0.02) &  0.51 (± 0.02) \\
CONEXP          &   0.5 (± 0.02) &   0.5 (± 0.02) &  0.39 (± 0.02) &  0.48 (± 0.02) \\
SLearner        &  0.43 (± 0.01) &  0.41 (± 0.02) &  0.35 (± 0.02) &   0.4 (± 0.02) \\
TCAV            &  1.59 (± 0.02) &  1.44 (± 0.02) &  1.72 (± 0.02) &  1.57 (± 0.02) \\
INLP            &  0.54 (± 0.02) &  0.69 (± 0.03) &  0.43 (± 0.04) &  0.57 (± 0.04) \\
ConceptShap     &  0.46 (± 0.02) &  0.46 (± 0.02) &  0.44 (± 0.01) &  0.47 (± 0.01) \\
CausaLM         &  0.51 (± 0.02) &  0.58 (± 0.02) &  0.41 (± 0.02) &  0.52 (± 0.01) \\
\bottomrule
\end{tabular}
\end{center}

\subsubsection{LSTM (5-way, ICaCE-normdiff)}
\begin{center}
\begin{tabular}{lllll}
\toprule
{} &       ambiance &           food &          noise &        service \\
\midrule
RandomExplainer &  0.62 (± 0.01) &  0.68 (± 0.01) &  0.53 (± 0.02) &  0.62 (± 0.01) \\
CONEXP          &  0.61 (± 0.01) &   0.61 (± 0.0) &  0.52 (± 0.02) &   0.6 (± 0.01) \\
SLearner        &  0.56 (± 0.01) &   0.54 (± 0.0) &  0.49 (± 0.02) &  0.53 (± 0.01) \\
TCAV            &   1.5 (± 0.02) &  1.38 (± 0.01) &  1.62 (± 0.02) &  1.49 (± 0.01) \\
INLP            &  0.62 (± 0.02) &  0.62 (± 0.01) &  0.54 (± 0.02) &   0.6 (± 0.01) \\
ConceptShap     &   0.56 (± 0.0) &   0.5 (± 0.01) &  0.58 (± 0.01) &  0.56 (± 0.01) \\
CausaLM         &  0.73 (± 0.02) &  0.86 (± 0.01) &  0.61 (± 0.02) &  0.74 (± 0.01) \\
\bottomrule
\end{tabular}
\end{center}

\subsubsection{roberta-base (5-way, ICaCE-normdiff)}
\begin{center}
\begin{tabular}{lllll}
\toprule
{} &       ambiance &           food &          noise &        service \\
\midrule
RandomExplainer &  0.69 (± 0.01) &  0.79 (± 0.01) &  0.63 (± 0.01) &   0.7 (± 0.01) \\
CONEXP          &  0.68 (± 0.01) &   0.7 (± 0.01) &  0.62 (± 0.02) &  0.66 (± 0.01) \\
SLearner        &  0.59 (± 0.01) &    0.6 (± 0.0) &  0.56 (± 0.02) &  0.57 (± 0.01) \\
TCAV            &  1.44 (± 0.01) &  1.27 (± 0.01) &  1.53 (± 0.02) &  1.43 (± 0.01) \\
INLP            &  0.77 (± 0.01) &  0.92 (± 0.01) &  0.69 (± 0.02) &  0.78 (± 0.01) \\
ConceptShap     &  0.62 (± 0.01) &  0.61 (± 0.01) &   0.6 (± 0.01) &  0.62 (± 0.01) \\
CausaLM         &   0.7 (± 0.01) &  0.82 (± 0.01) &  0.64 (± 0.01) &  0.72 (± 0.01) \\
\bottomrule
\end{tabular}
\end{center}
